# Supplementary material for: Acquisition of Spatially-Varying Reflectance and Surface Normals via Polarized Reflectance Fields
Source: arXiv:2412.09772 source file (2024-12-13)
Supplement: Supplementary file 1 [file Supp_Qualitative.tex]

\begin{figure*}[h]
    \centering
    \includegraphics[width=\linewidth]{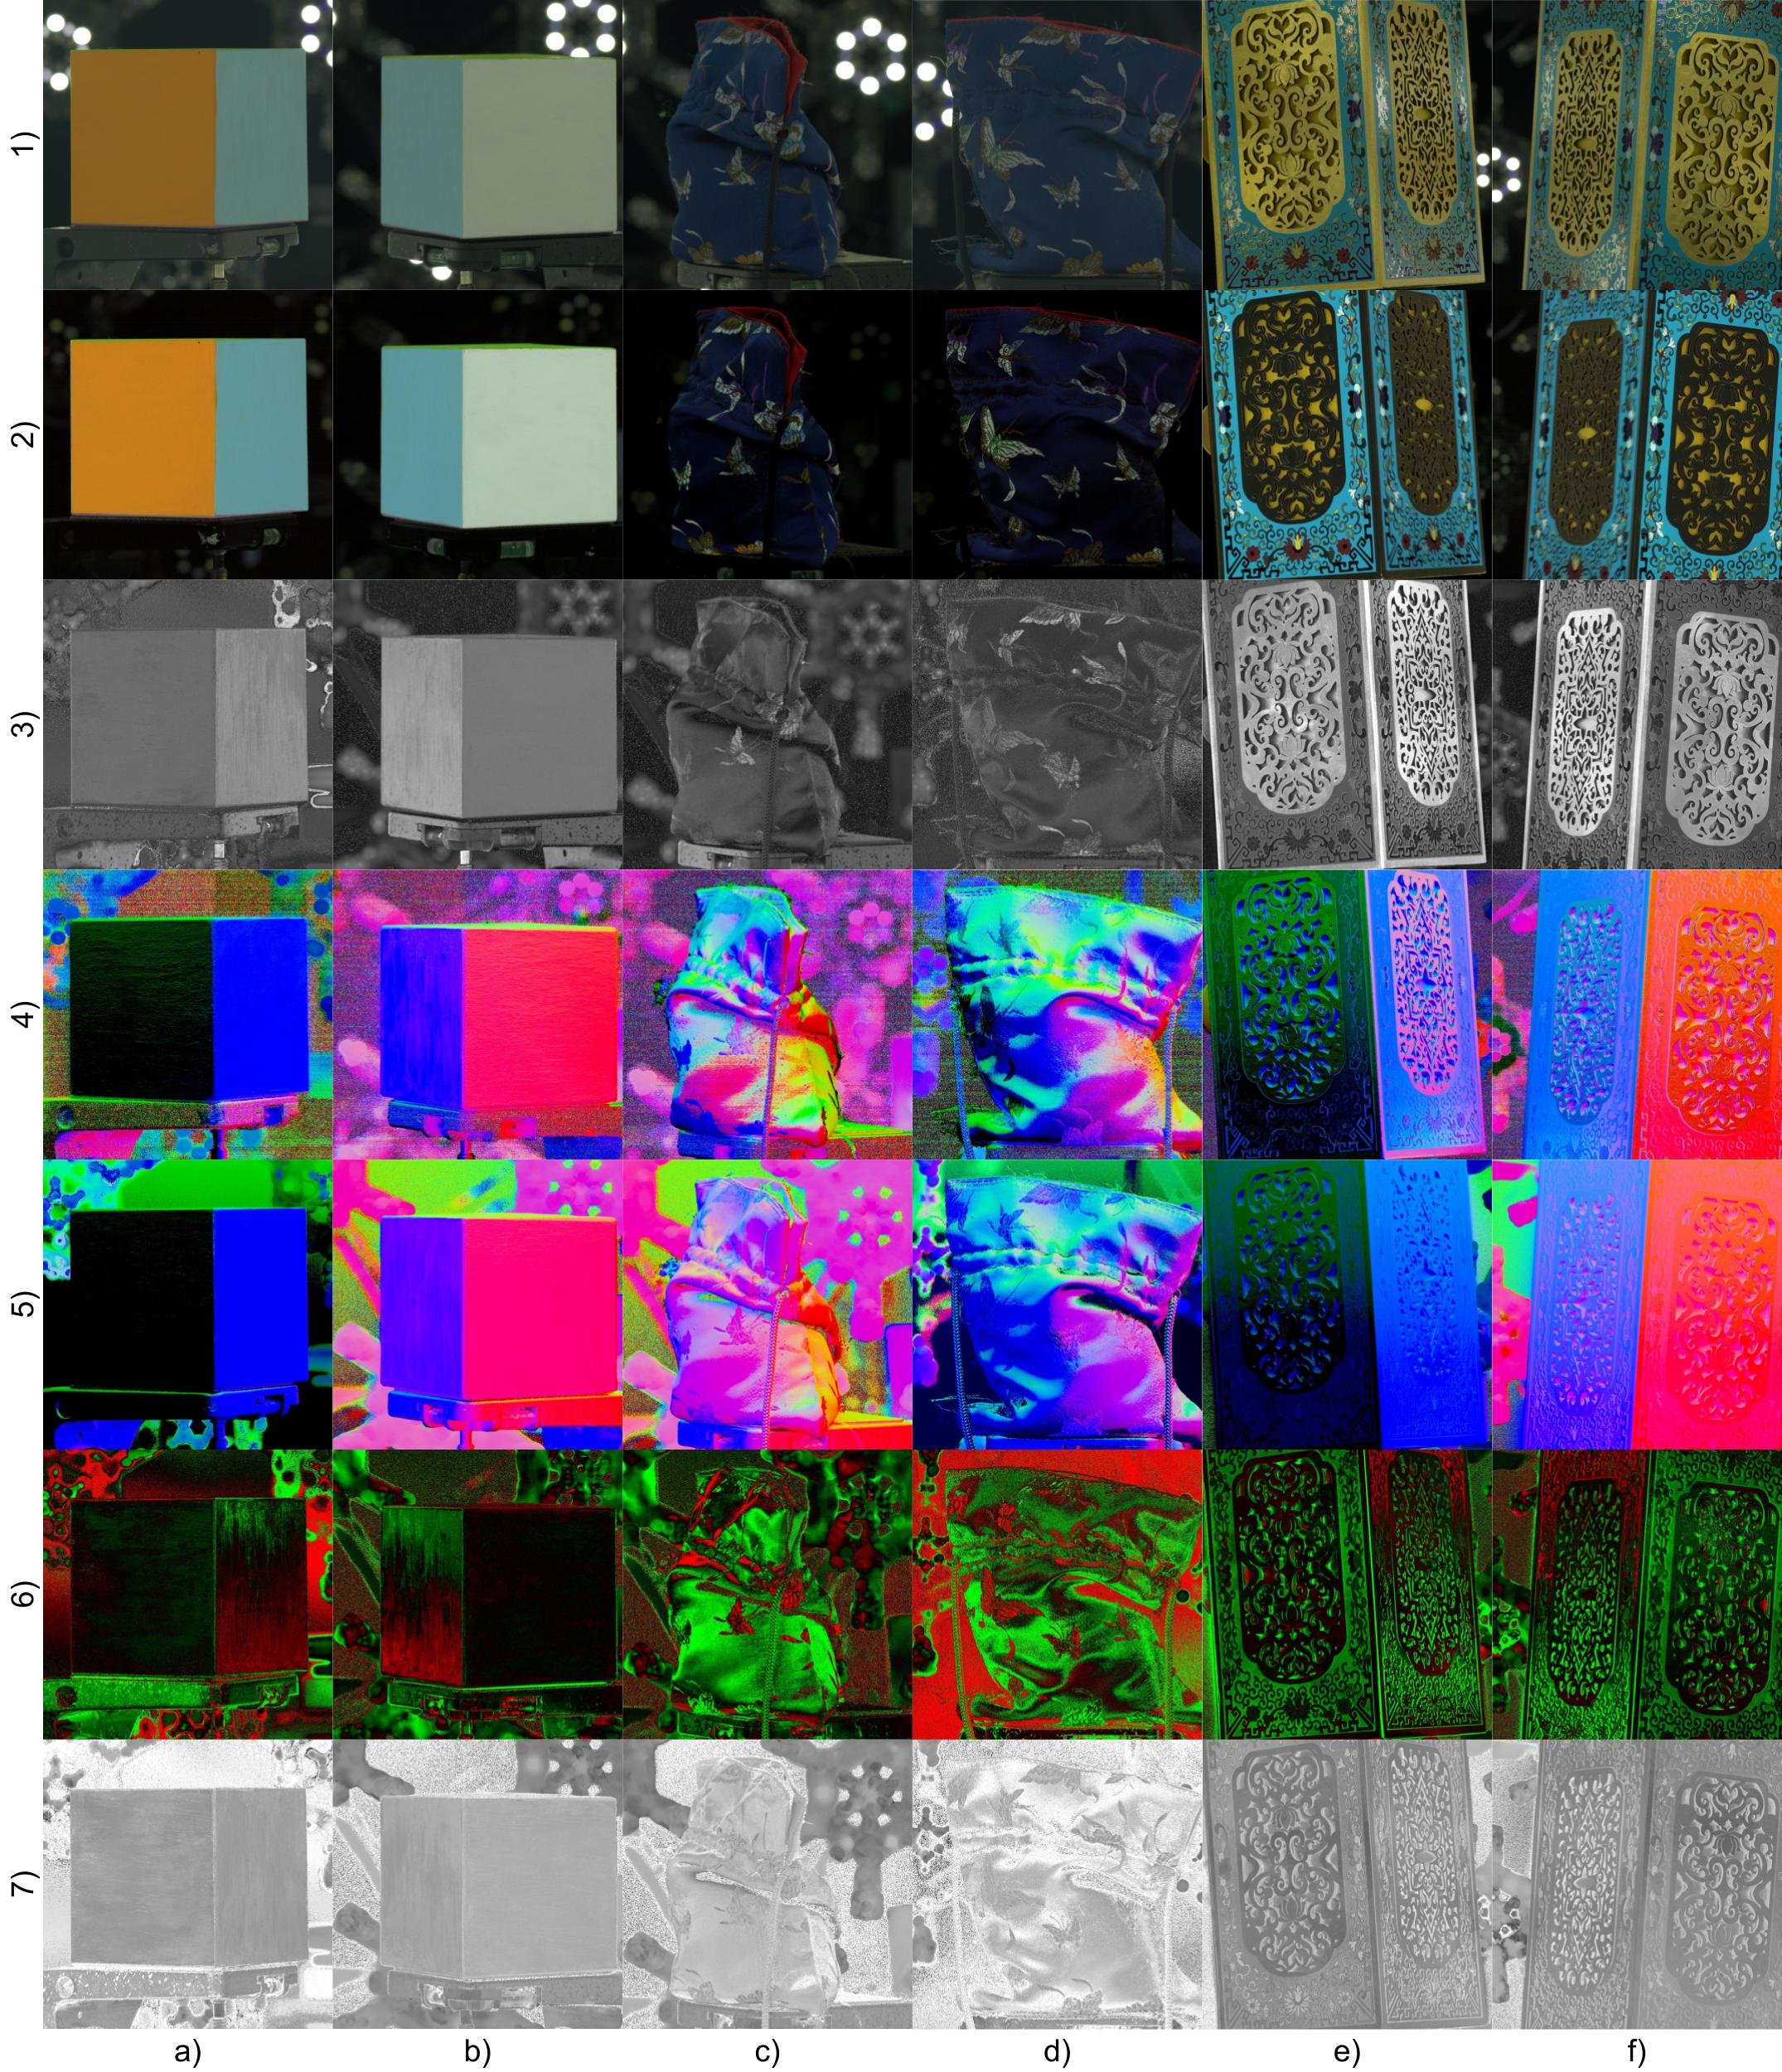}
    \caption{\textbf{More Optimization Results.} We present a wooden painted cube from a) left and b) right, a fabric bag from c) right and d) front, and a gift box from e) left and f) right. For each object, we showcase 1) original image, 2) diffuse albedo $\hat{\rho}_d$, 3) specular albedo $\hat{\rho}_s$, 4) diffuse normal $\hat{n}_d$, 5) specular normal $\hat{n}_s$, 6) anisotropy $\varrho$, and 7) roughness $\gamma$.}
    \label{fig:supp_qualitative}
\end{figure*}
% https://docs.google.com/presentation/d/1MHPsaoRJKB4KSRbejoh7Y48wnkHT3NY7Jn2bLGdH2VA/edit?usp=sharing
